# Supplementary material for: Time-adaptive single-shot crosstalk detector on superconducting quantum computer
Source: arXiv:2502.14225 source file (2025-08-15)
Supplement: Supplementary file 1 [file Supplementary_Materials_for_Time_adaptive_single_shot_crosstalk_detector_on_superconducting_quantum_computer.pdf]

# Supplementary Materials for: Time-adaptive single-shot crosstalk detector on superconducting quantum computer

Dephasing and amplitude damping derived using  $T_1$  and  $T_2$  from *ibm\_torino*,  $\theta = \frac{\pi}{4}$  with maximum of 4 spectator qubits

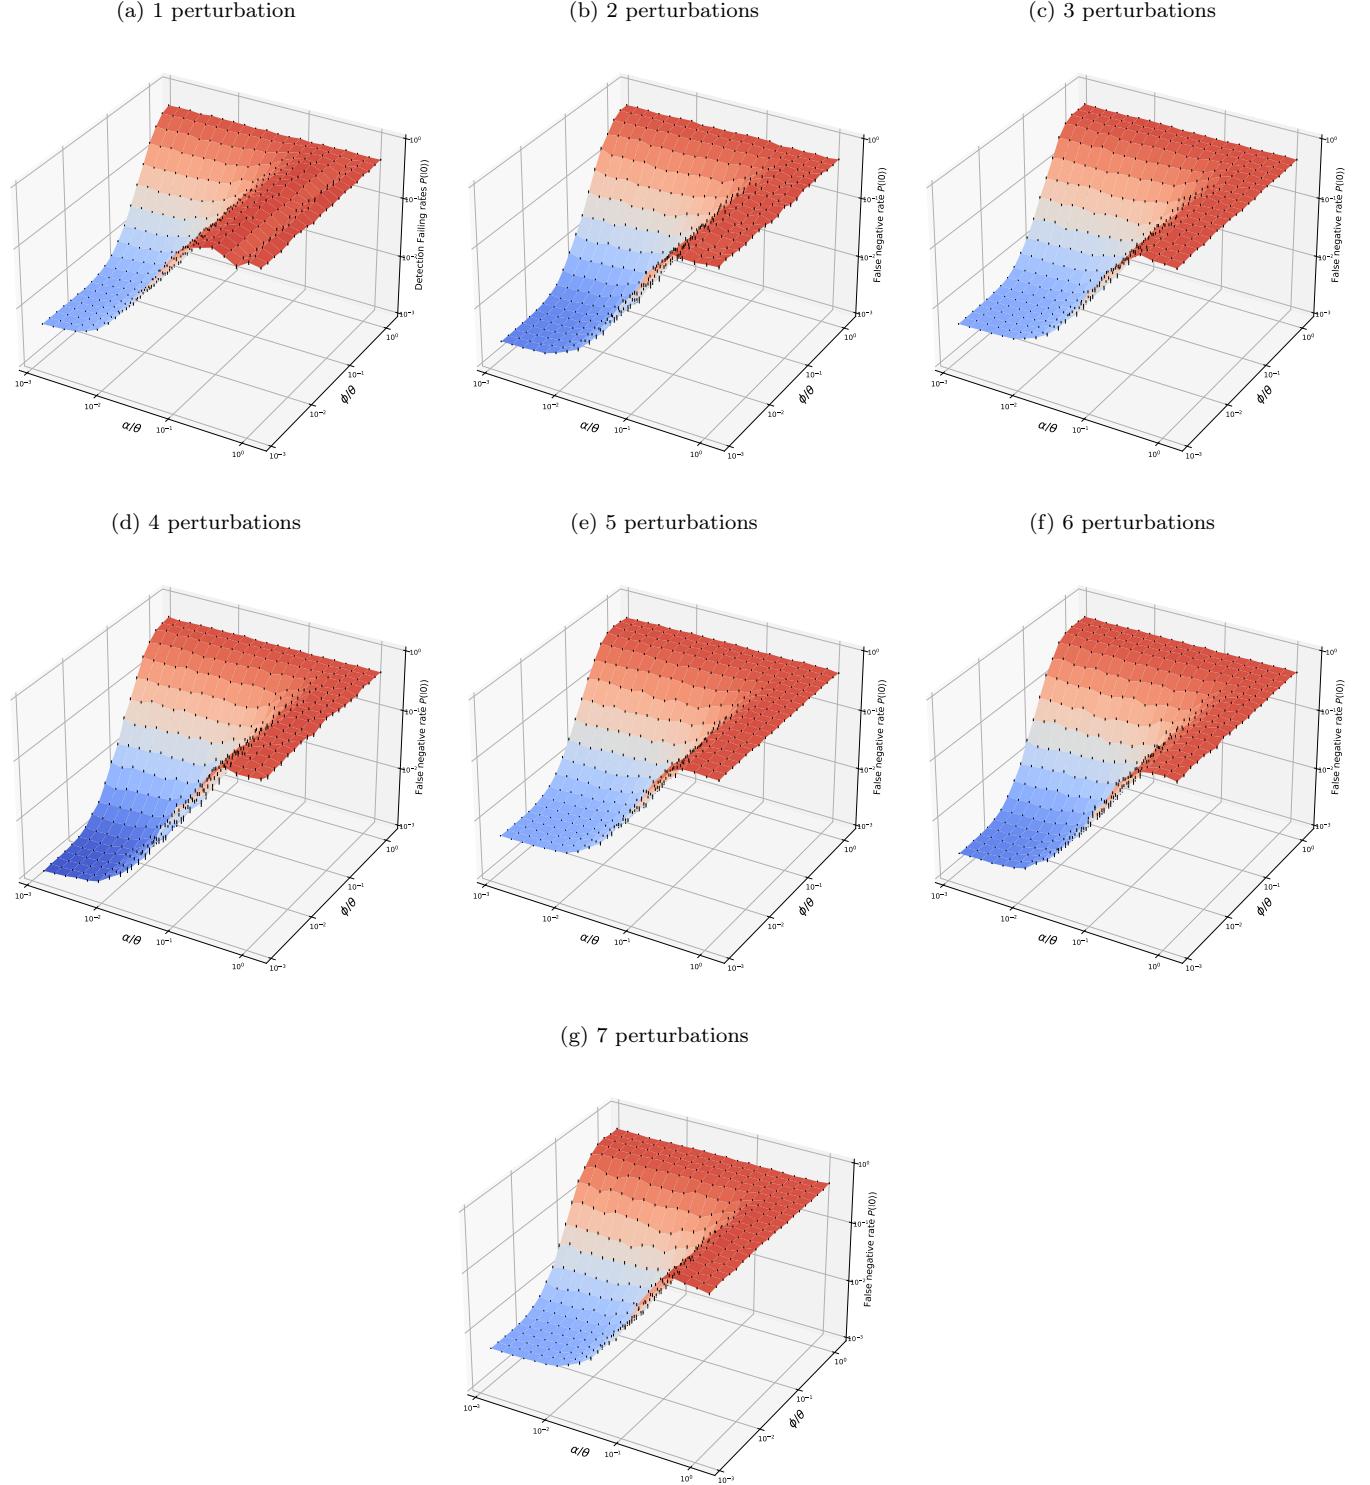

FIG. 1. The corresponding 3D surface plot to Figure 11a (from the main text) with error bars. The half-length of the error bars of each data point take two times the standard error sampled in 50 trials.

Dephasing and amplitude damping derived using  $T_1$  and  $T_2$  from *ibm\_sherbrooke*,  $\theta = \frac{\pi}{4}$  with maximum of 4 spectator qubits

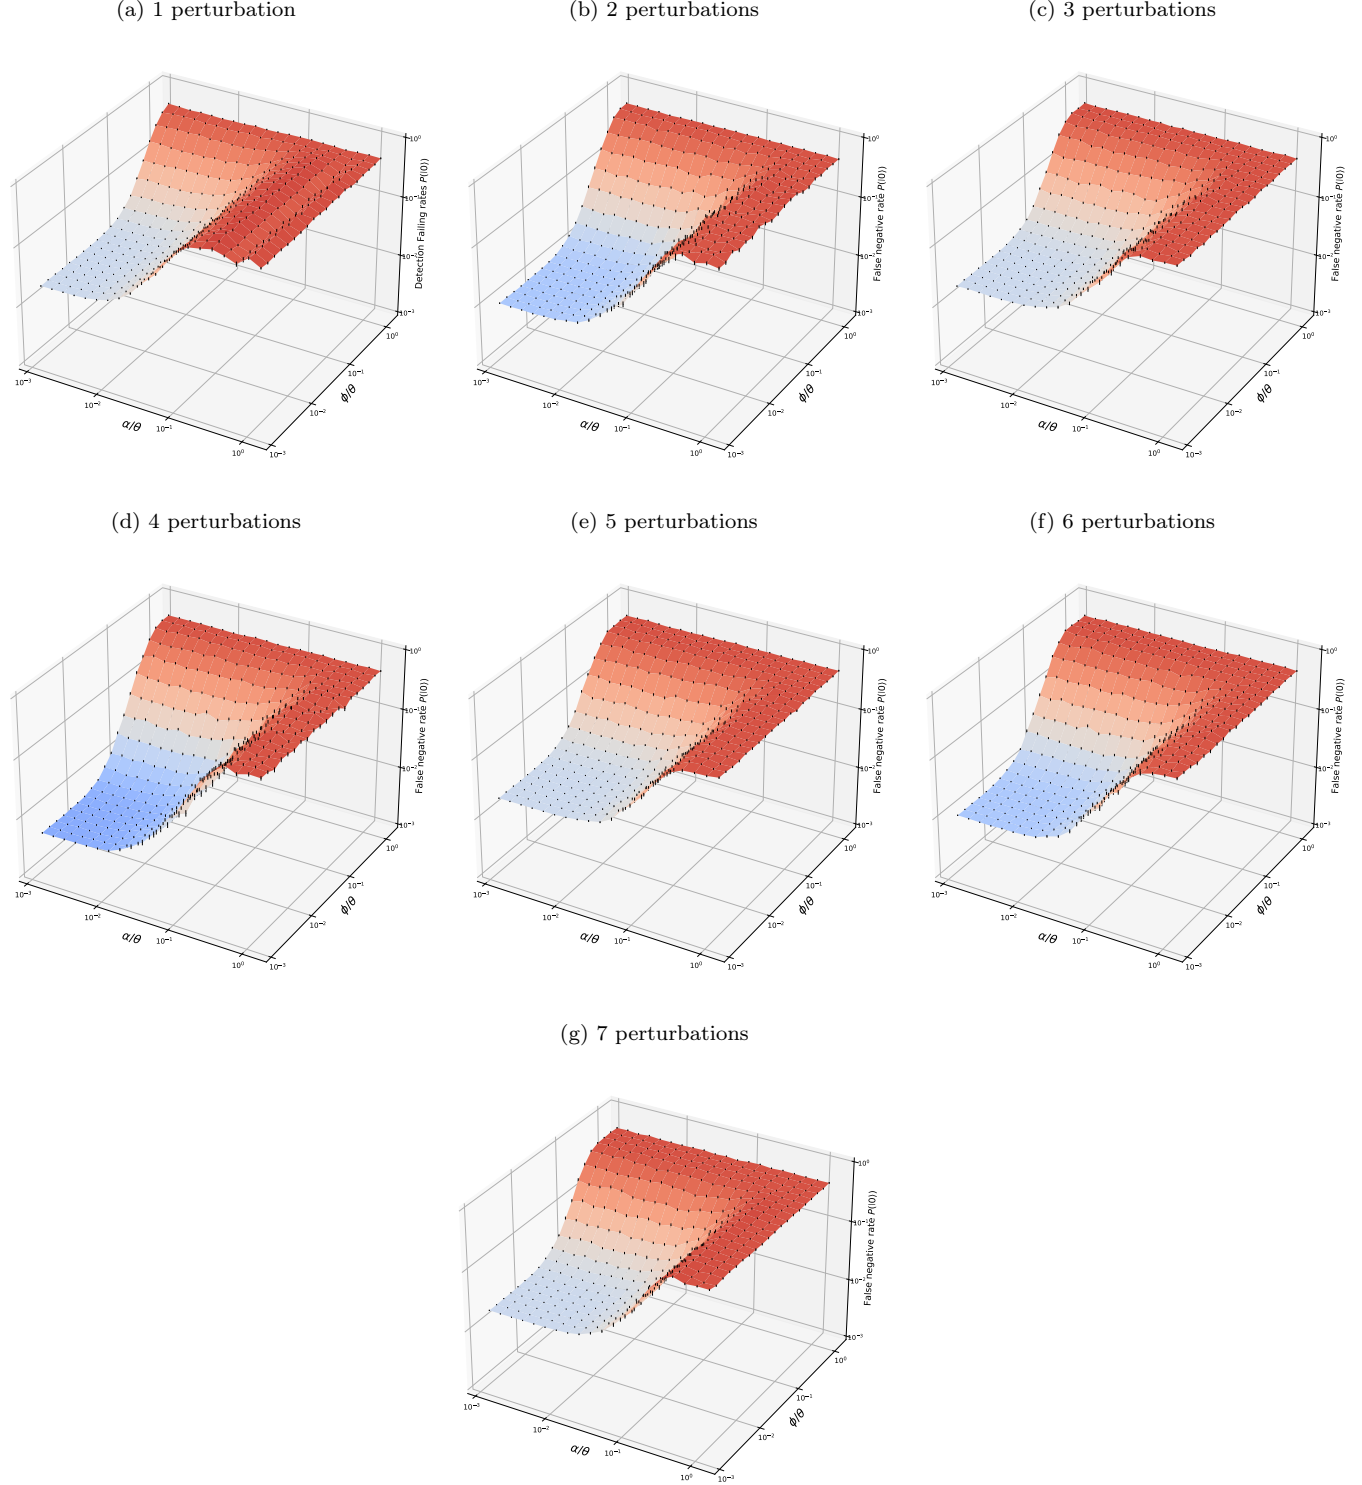

FIG. 2. The corresponding 3D surface plot to Figure 11b (from the main text) with error bars. The half-length of the error bars of each data point take two times the standard error sampled in 50 trials.

No dephasing and amplitude damping,  $\theta = \frac{\pi}{4}$  with maximum of 4 spectator qubits

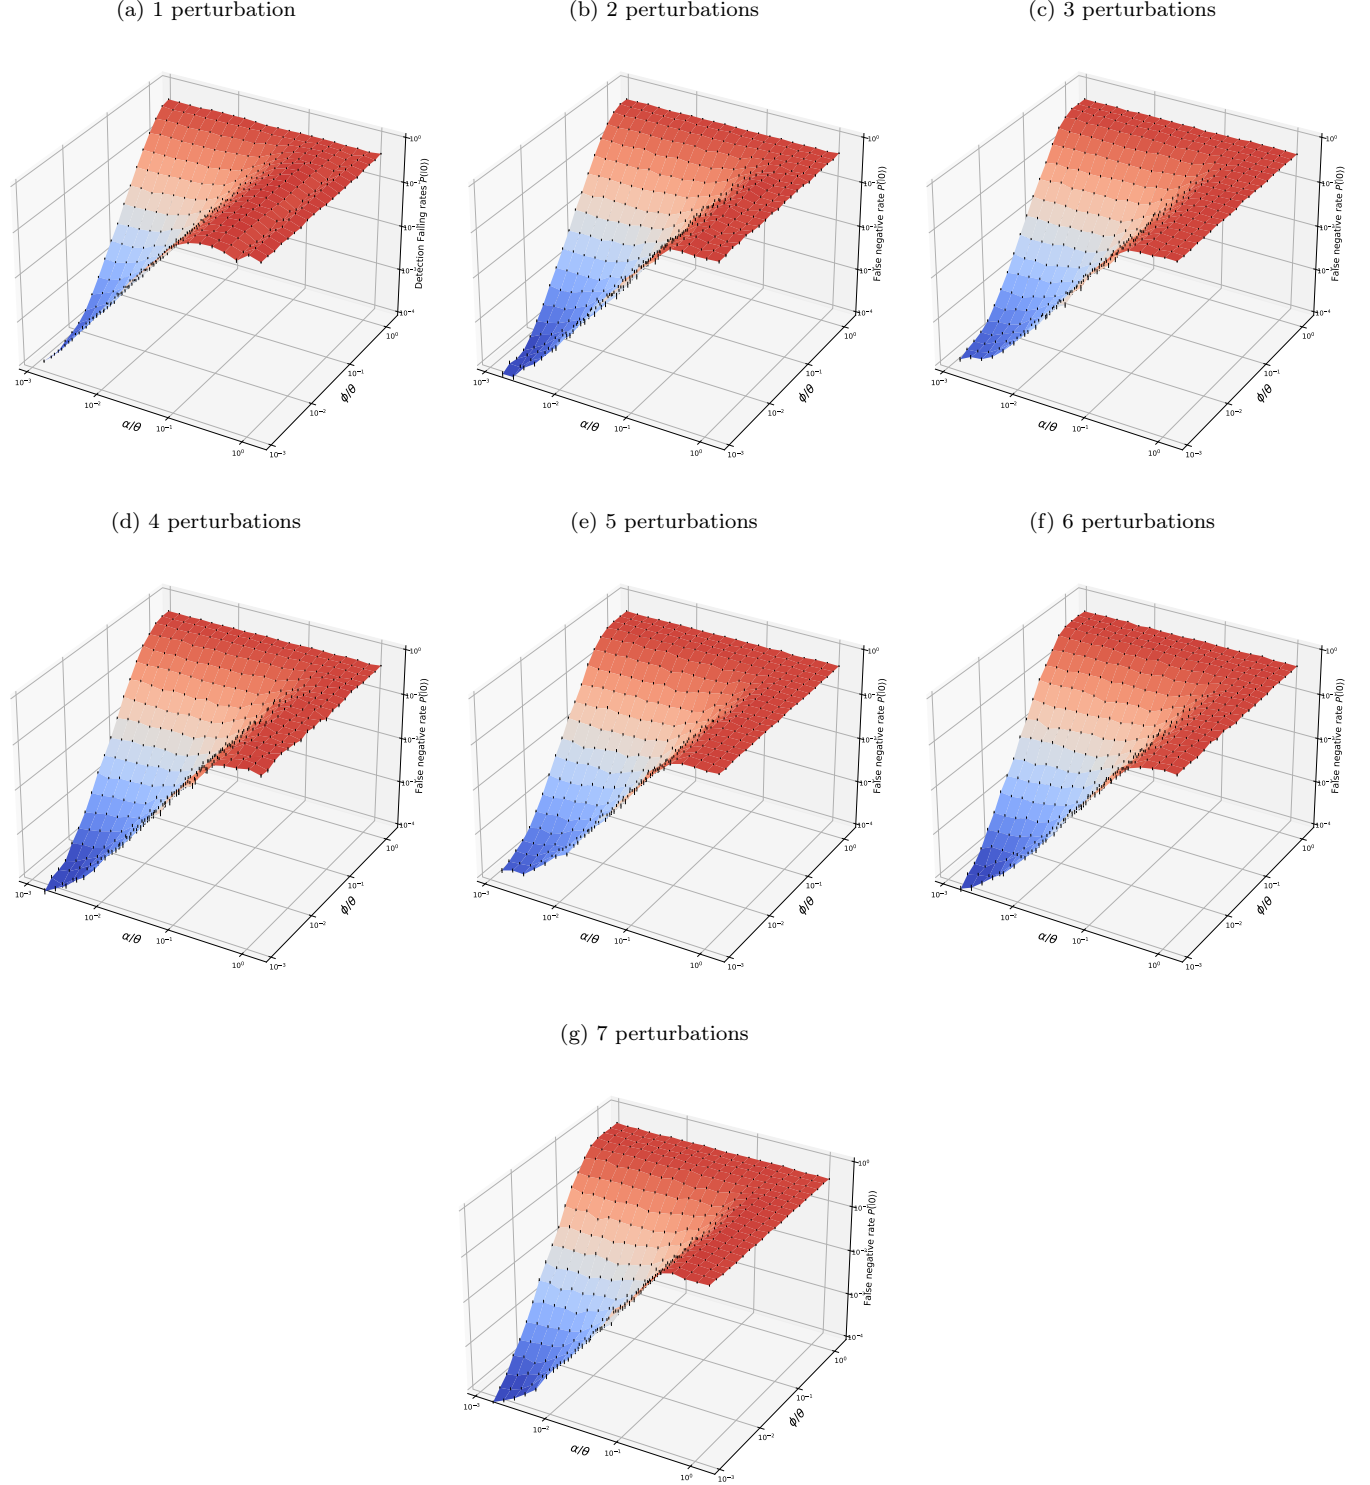

FIG. 3. The corresponding 3D surface plot to Figure 11c (from the main text) with error bars. The half-length of the error bars of each data point take two times the standard error sampled in 50 trials. Note that the minimum position of the colourscale is now  $10^{-4}$ .

$T_1$  and  $T_2$  from *ibm\_torino*,  $\theta = \frac{2\pi}{9}$  with maximum of 4 spectator qubits

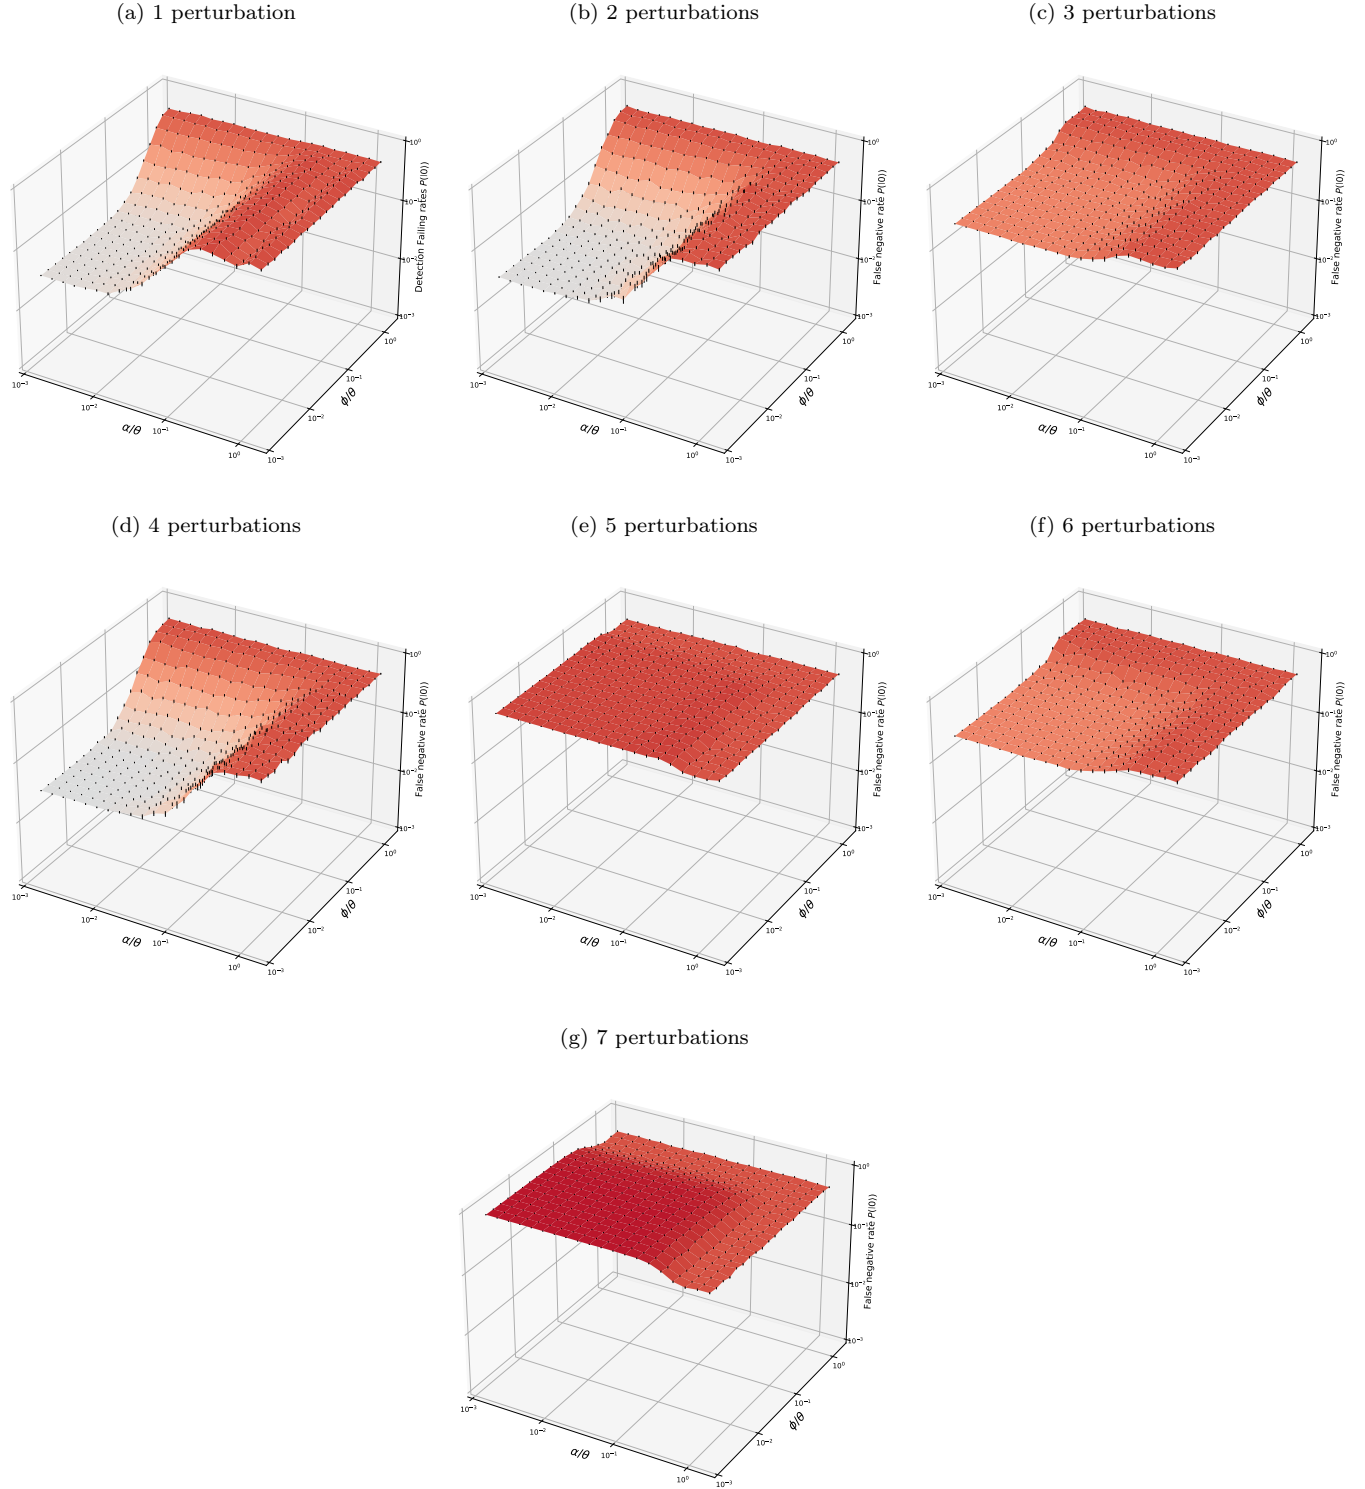

FIG. 4. The corresponding 3D surface plot to Figure 12a (from the main text) with error bars. The half-length of the error bars of each data point take two times the standard error sampled in 50 trials.

$T_1$  and  $T_2$  from *ibm\_sherbrooke*,  $\theta = \frac{2\pi}{9}$  with maximum of 4 spectator qubits

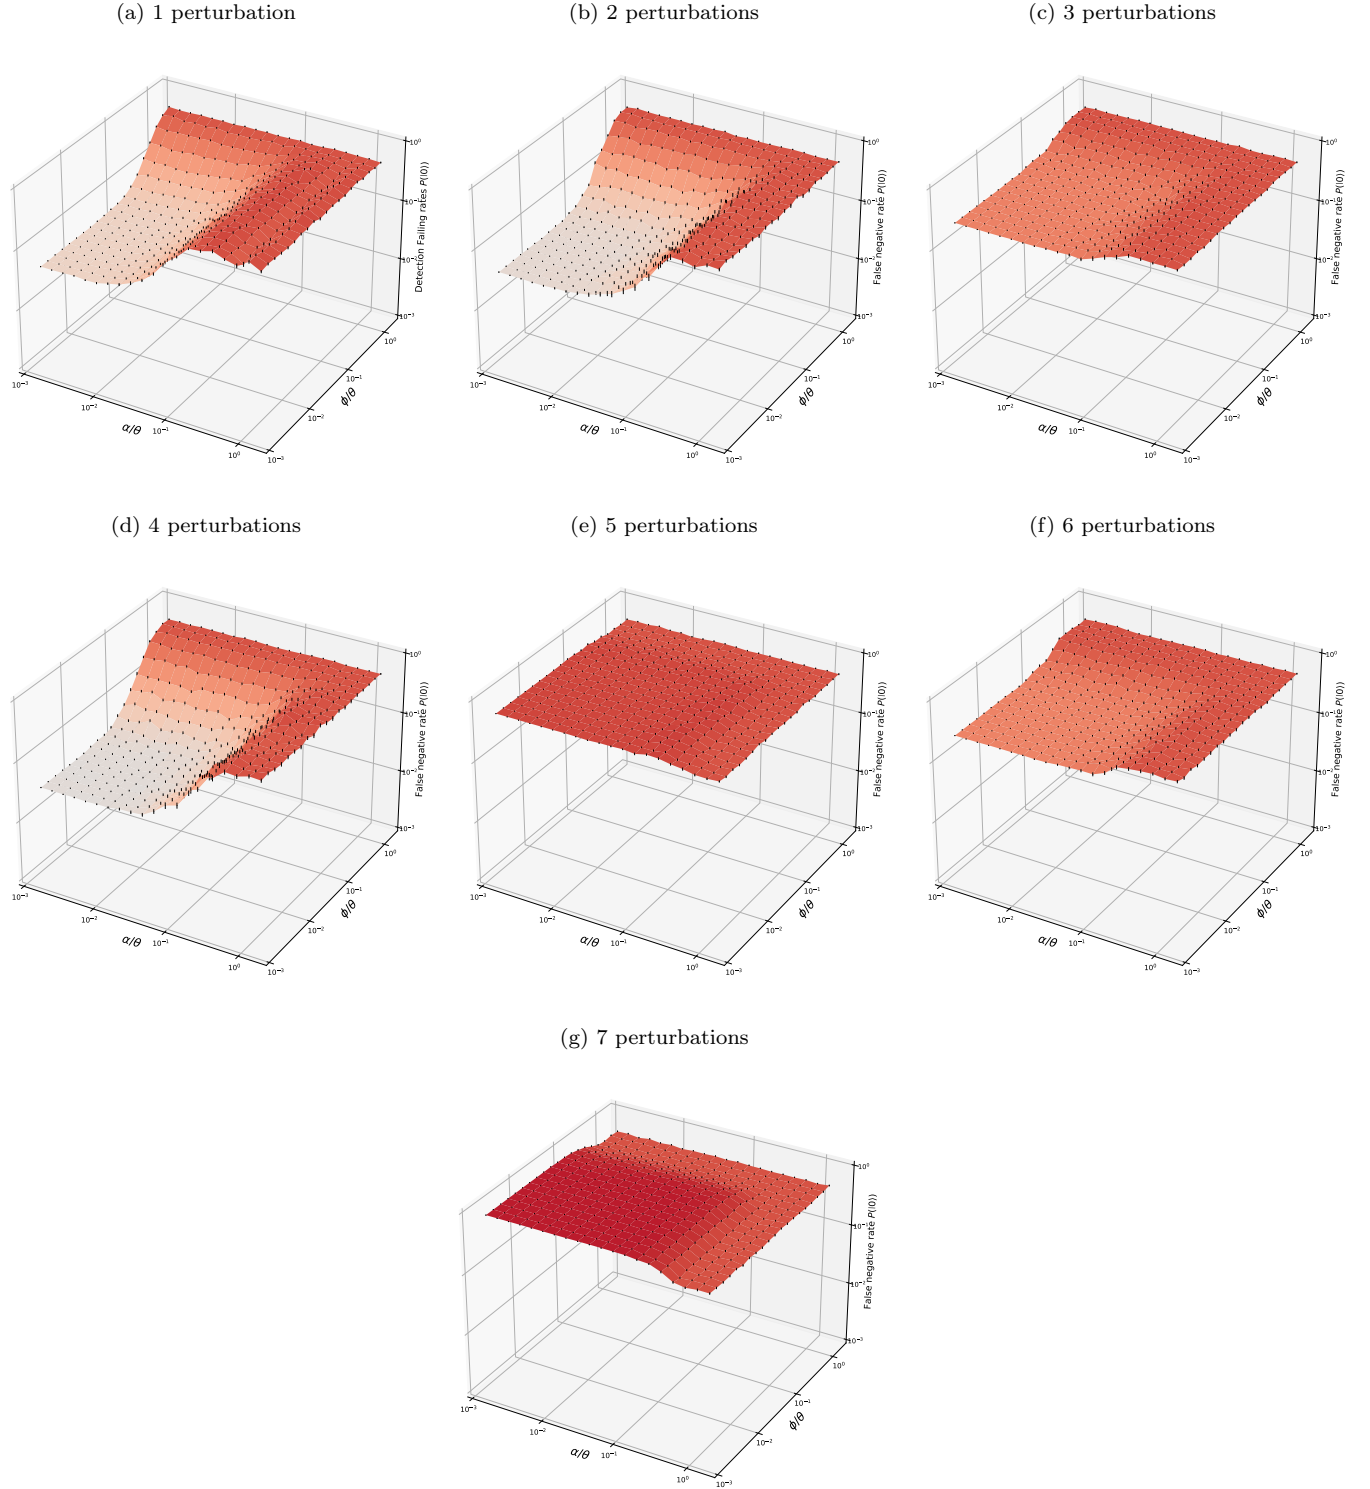

FIG. 5. The corresponding 3D surface plot to Figure 12b (from the main text) with error bars. The half-length of the error bars of each data point take two times the standard error sampled in 50 trials.

No dephasing and amplitude damping,  $\theta = \frac{2\pi}{9}$  with maximum of 4 spectator qubits

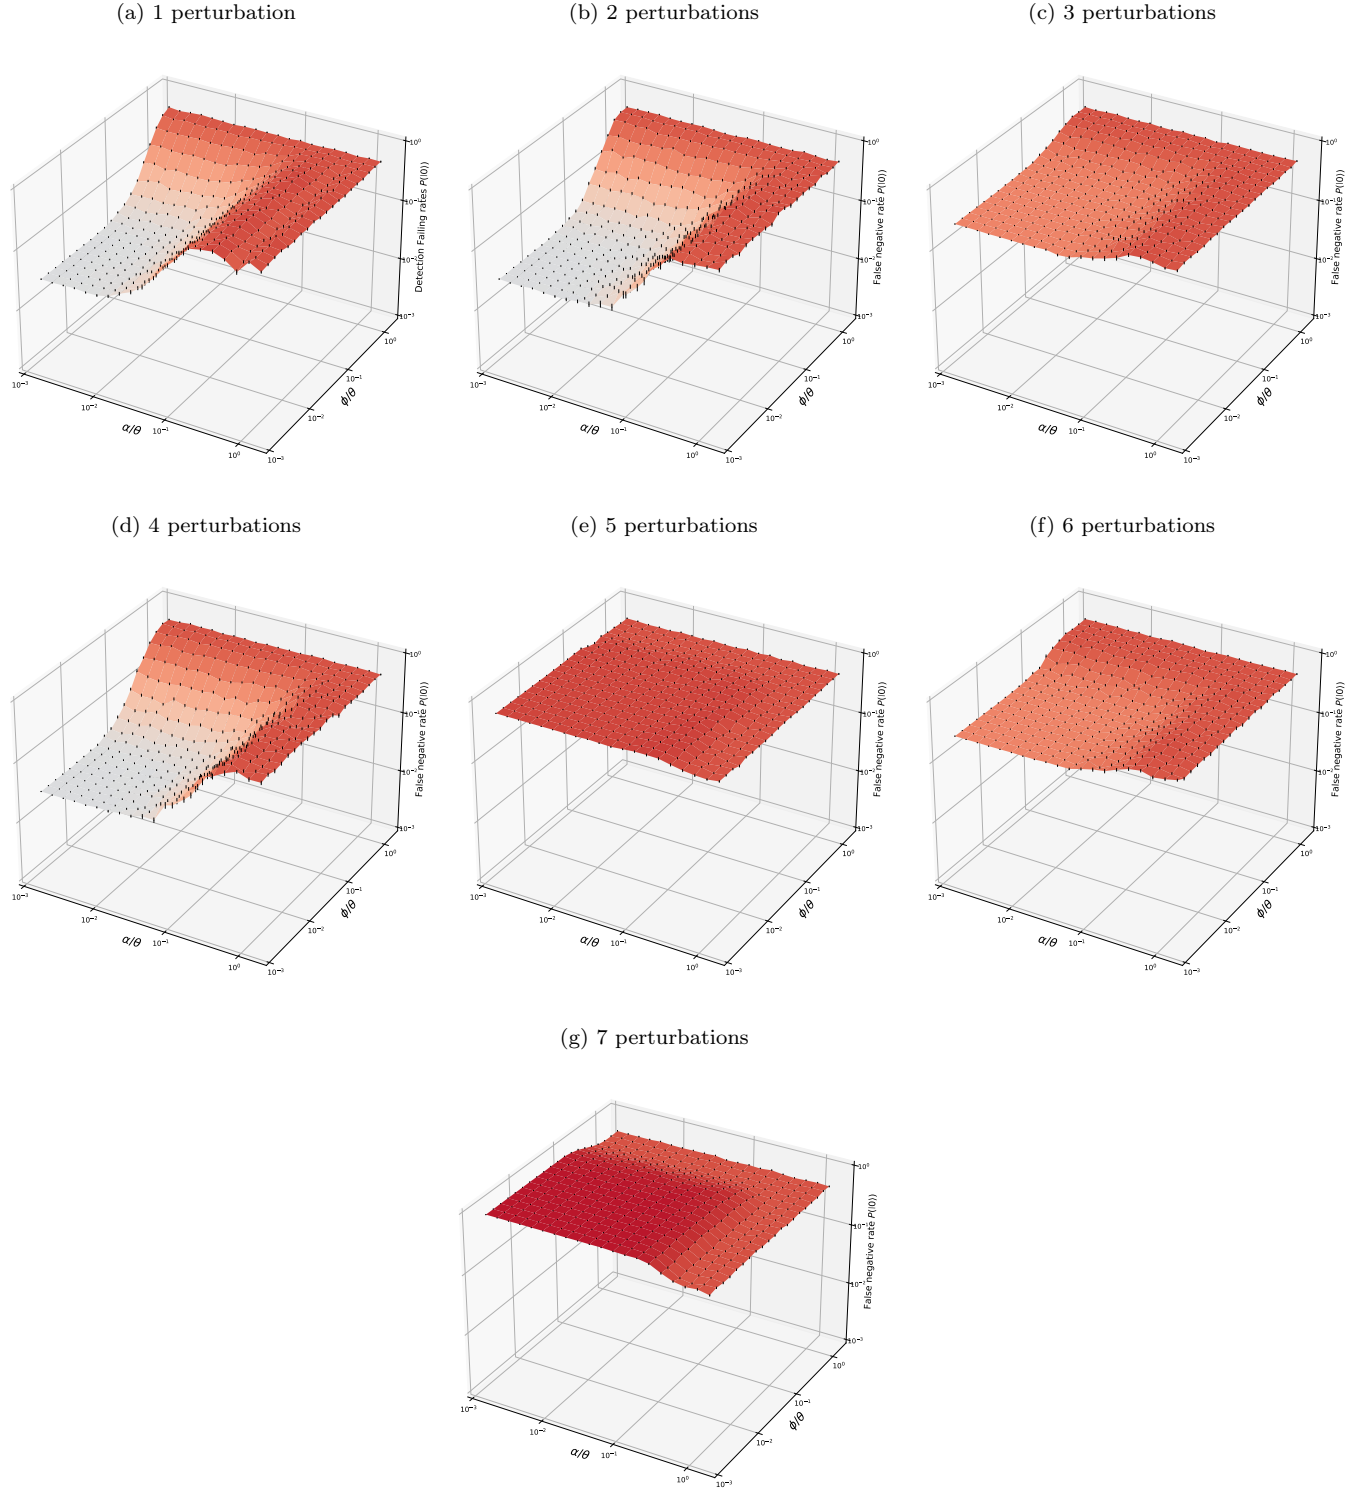

FIG. 6. The corresponding 3D surface plot to Figure 12c (from the main text) with error bars. The half-length of the error bars of each data point take two times the standard error sampled in 50 trials.



No dephasing and amplitude damping,  $\theta = \frac{\pi}{8}$  with maximum of 8 spectator qubits

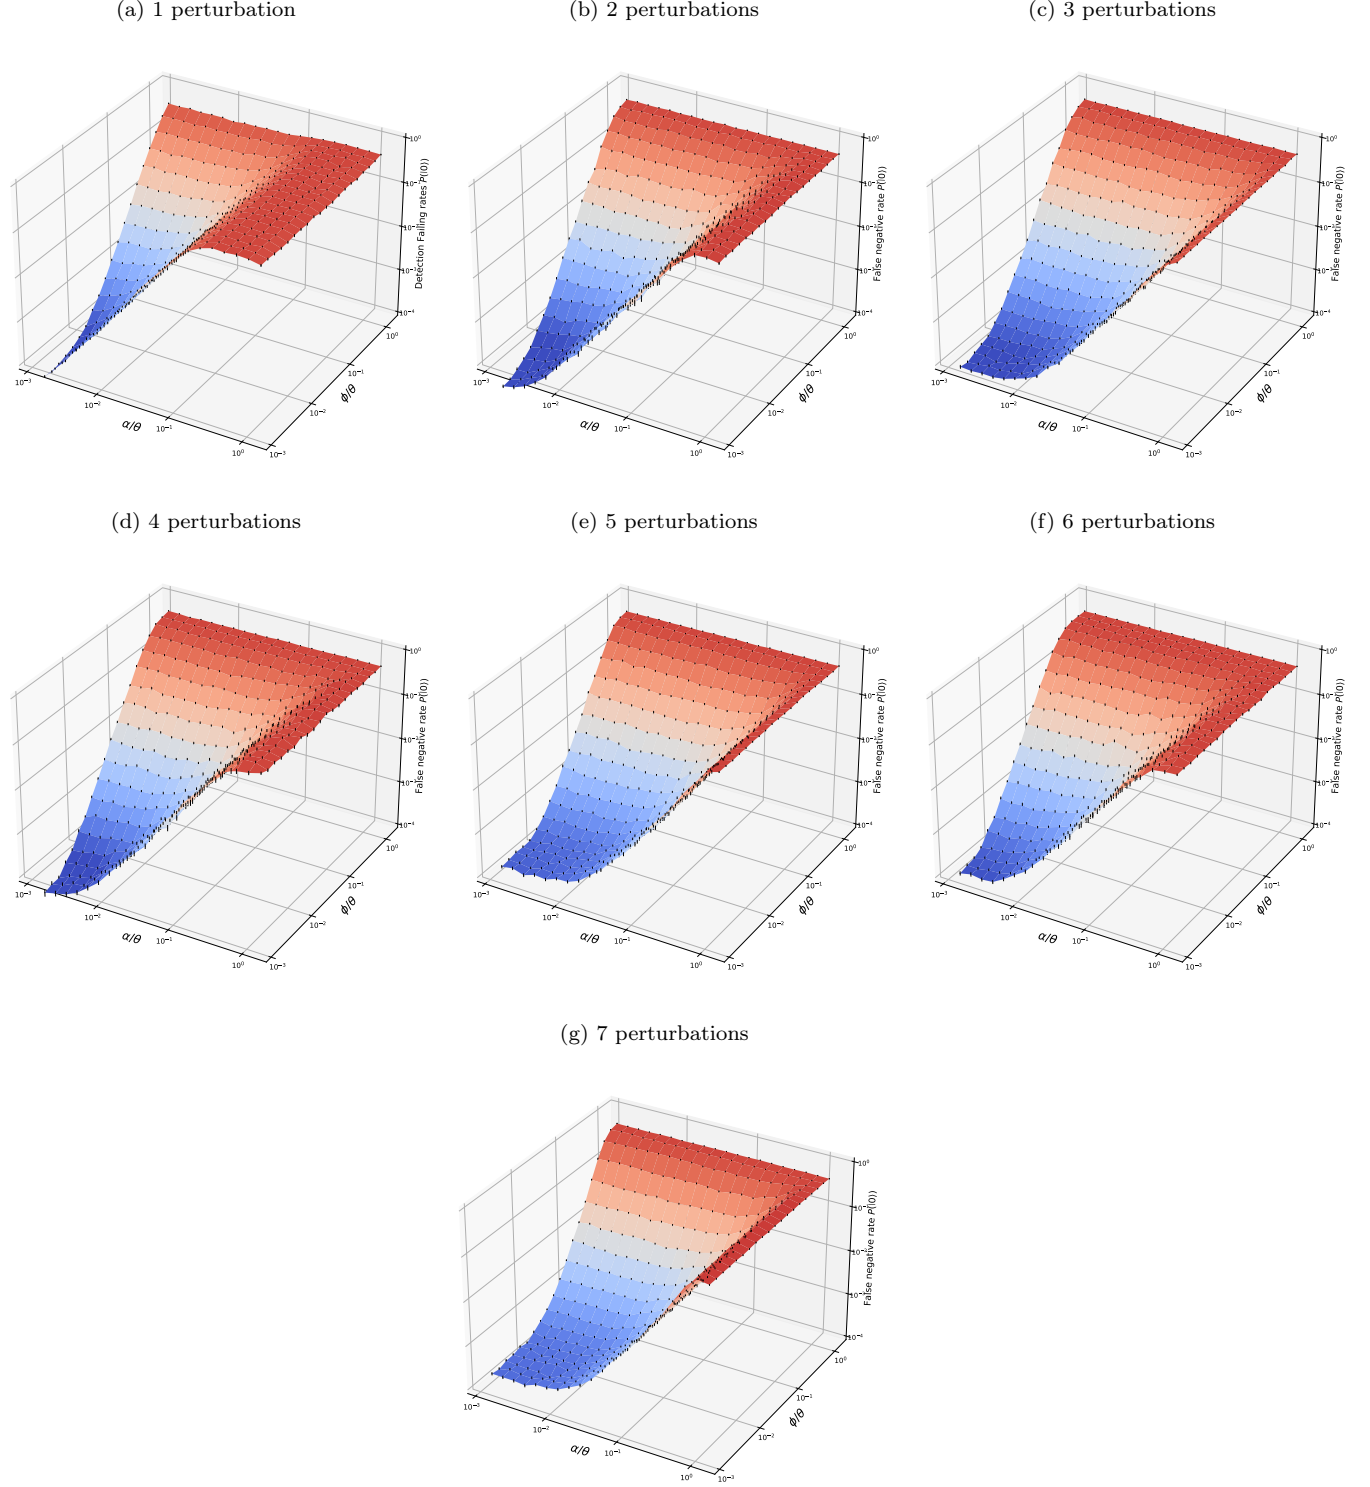

FIG. 7. The corresponding 3D surface plot to Figure 13 (from the main text) with error bars. The half-length of the error bars of each data point take two times the standard error sampled in 50 trials.

No dephasing and amplitude damping,  $\theta = \frac{2\pi}{17}$  with maximum of 8 spectator qubits

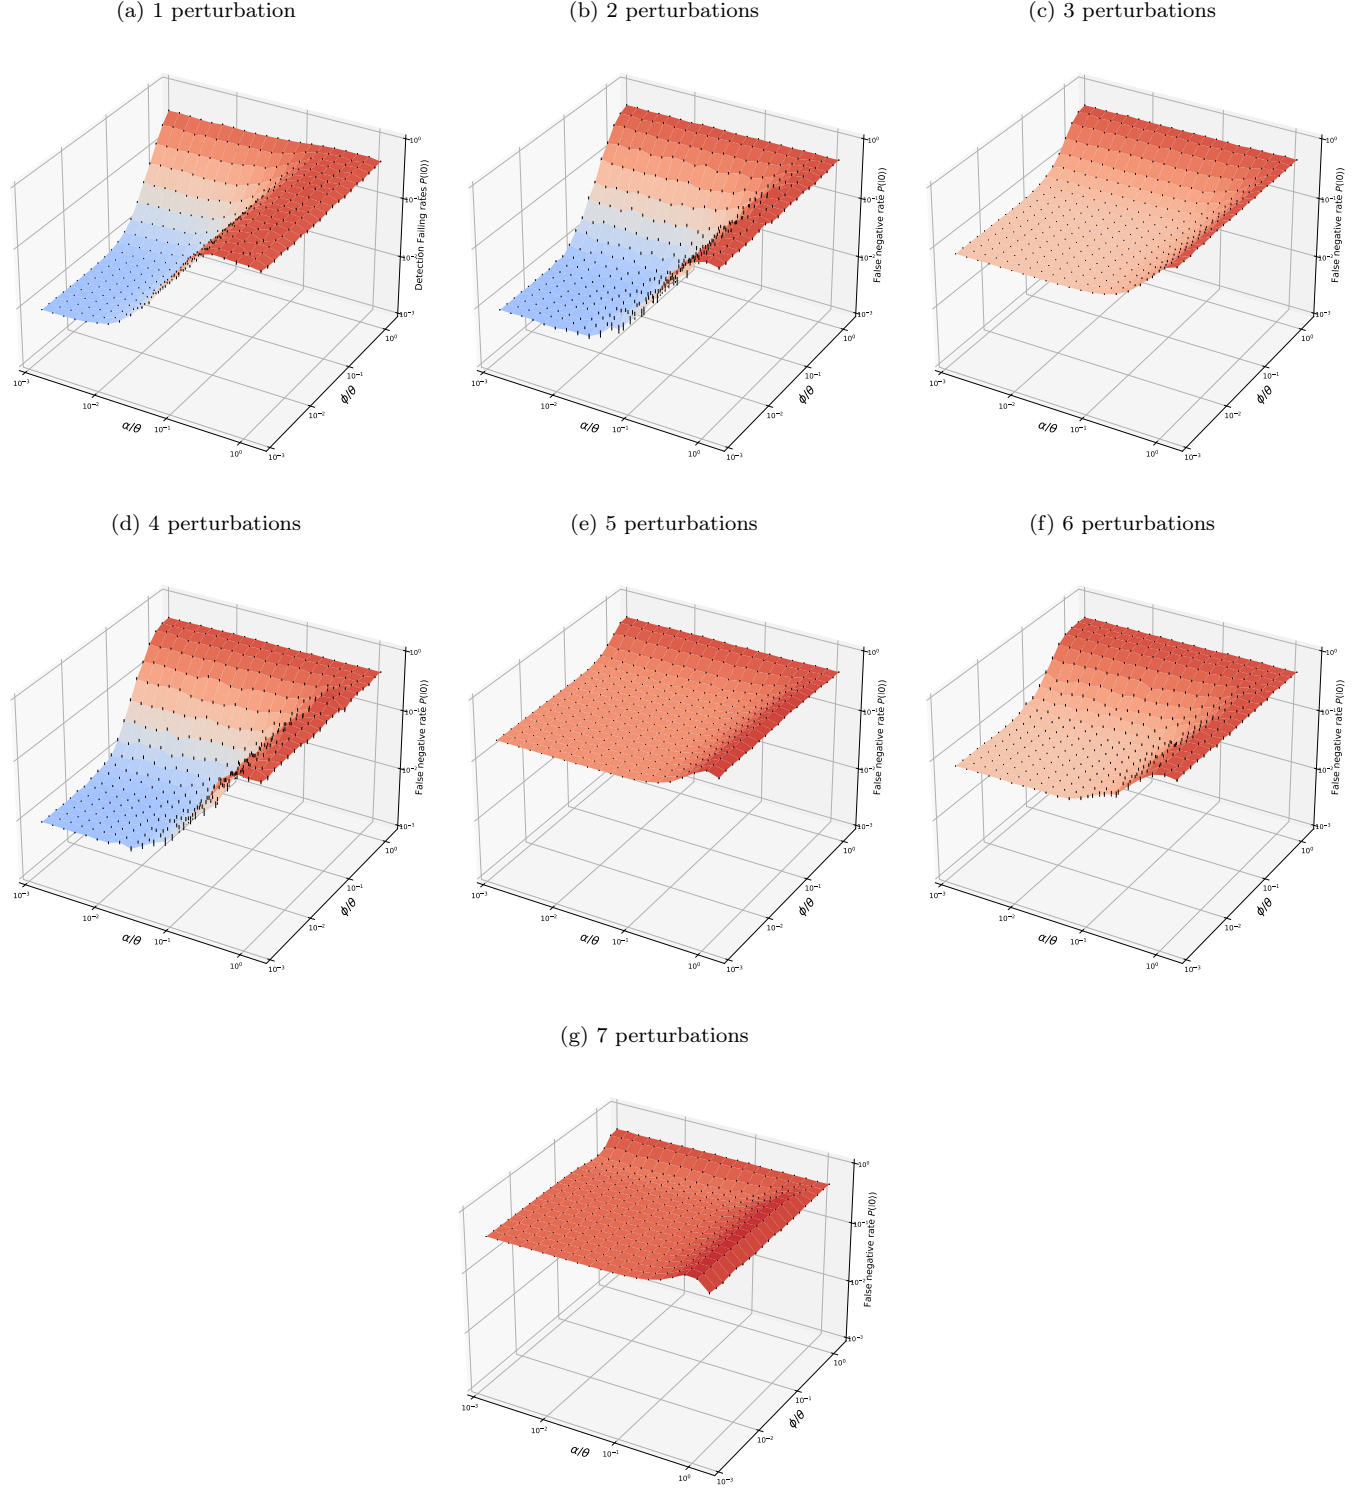

FIG. 8. The corresponding 3D surface plot to Figure 14 (from the main text) with error bars. The half-length of the error bars of each data point take two times the standard error sampled in 50 trials.
